# Supplementary material for: Model-Invariant State Abstractions for Model-Based Reinforcement Learning
Source: arXiv:2102.09850 source file (2021-06-07)
Supplement: Supplementary file 1 [file Appendix.tex]

\part*{Appendix}

\begin{theorem}
For the abstraction $\phi_{i}(x) = [x]_{S_{i}}$, where $S_{i}= \ $\textbf{PA($X_{i}^{t+1}$)}, $\phi$ is model-ICP-irrelevant. Furthermore, rather trivially, if $\phi(x^1) = \phi(x^2)$, for any $x^1, x^2 \sim \mathcal{X}$, we have
\begin{equation}
\label{eq: theorem1}
    \sum_{x^{\prime} \in \phi^{-1}(\bar{x})} P(x^{\prime} | x^{1}, a) = \sum_{x^{\prime} \in \phi^{-1}(\bar{x})} P(x^{\prime} | x^{2}, a)
\end{equation}
\end{theorem}

Note that the latter statement of Theorem 1 is a trivial result if we follow Theorem 1 in \cite{zhang2020invariant}. This is since, the condition $\phi(x^1) = \phi(x^2)$ is quite strict if we assume the absence of irrelevant state variables (If no such variables are present, then $x^1$ has to be equal to $x^2$ for such a condition to be met, which is not interesting). With such a strict condition over the abstraction over two states, each term in the LHS is equal to each term in the RHS of \ref{eq: theorem1}, i.e. 

\begin{equation}
    P(x^{\prime} | x^{1}, a) = P(x^{\prime} | x^{2}, a)
\end{equation}

However, in the general case, where there are irrelevant variables present, this definition makes more sense. On the other hand, the condition present in~\ref{def: model-ICP-irrelevance} is based on a particular index $i$ and is thus much less strict.

\emph{Proof.} We first prove the second statement. Given $\phi(x^1) = \phi(x^2)$, we have $\phi_{i}(x^1) = \phi_{i}(x^2)$ for each dimension $i$. Also,

\begin{center}
$P(x^{\prime} | x^{1}, a) = {\displaystyle \prod_{i=0}^{p}} P(x^{\prime}_{i} | x^{1}, a)
                        = {\displaystyle \prod_{i=0}^{p}} P(x^{\prime}_{i} | [x^1]_{S_{i}}, a)$ \\ 
                        \hspace{-1cm} $= {\displaystyle \prod_{i=0}^{p}} P(x^{\prime}_{i} | \phi_{i}(x^1), a)$
\end{center}

Similarly, $P(x^{\prime} | x^{2}, a) = {\displaystyle \prod_{i=0}^{p}} P(x^{\prime}_{i} | \phi_{i}(x^2), a)$ and since $\phi_{i}(x^1) = \phi_{i}(x^2)$, we have $P(x^{\prime} | x^{1}, a) = P(x^{\prime} | x^{2}, a)$.

Now, in the case where $\phi_{i}(x^1) = \phi_{i}(x^2)$ for a specific dimension $i$, we have:

\begin{center}
\hspace{-5.5cm} ${\displaystyle \sum_{x^{\prime} \in \phi_{i}^{-1}(\bar{x})}} P(x^{\prime} | x^{1}, a) = {\displaystyle \sum_{x^{\prime} \in \phi_{i}^{-1}(\bar{x})}} \ {\displaystyle \prod_{k=0}^{p}} P(x^{\prime}_{k} | x^{1}, a) $ \\
$ = {\displaystyle \sum_{x^{\prime} \in \phi_{i}^{-1}(\bar{x})}} P(x^{\prime}_{i} | [x^1]_{S_{i}}, a) \  {\displaystyle \prod_{k=0}^{p}} P(x^{\prime}_{k \neq i} | x^{1}, a)$ \\
\hspace{-0.2cm}$ = P(x^{\prime}_{i} | \phi_{i}(x^1), a) {\displaystyle \sum_{x^{\prime} \in \phi_{i}^{-1}(\bar{x})}} \ P([x^{\prime}]_{k \neq i} | x^{1}, a)$ \\
\hspace{-4cm} $ = P(x^{\prime}_{i} | \phi_{i}(x^1), a) $ \\
\hspace{-4cm} $ = P(x^{\prime}_{i} | \phi_{i}(x^2), a) $ 
\end{center}

Following the same steps backwards concludes the proof.
